# Supplementary material for: PASCL: Supervised Contrastive Learning with Perturbative Augmentation for Particle Decay Reconstruction
Source: arXiv:2402.11538 source file (2024-02-18)
Supplement: Supplementary file 1 [file appendix.tex]

\subsection{Lowest Common Ancestor Generation (LCAG) matrix}\label{subsec:LCAG}

Given two nodes in a graph, $a$ and $b$, the lowest common ancestor of them is defined as the deepest node that is an ancestor of both \sw{node} $a$ and \sw{node} $b$. \sw{Here, we refer to the farthest node from the root node $r$ as the deepest node. Formally, we define LCA as below:}
% deepest here means farthest from the root node $r$. Formally:
\begin{equation}
\begin{aligned}
&{\tiny \mathrm{LCA}(a,b)} =\\
&{\tiny \mathrm{argmax}_p\{dist(p,r)|p\in\mathrm{path}(a,r)\wedge p\in\mathrm{path}(b,r) \}.}
\end{aligned}
\end{equation}

In order to \sw{transform} the LCA matrix into a format \sw{that is dedicated to the process of our proposed deep learning method, }
% suitable for end-to-end training 
% for machine learning\inote{ML is weird. (Solved)}, 
we \sw{set reconstructing the ground truth LCAG matrix as our objective. }
% use the LCAG matrix to represent our learning target\inote{You did not use LCAG to solve the problem, you use it to represent data! (Solved)}. 
In the LCAG matrix, each entry of the LCA matrix is replaced with its corresponding generation in the tree. The LCAG matrix follows a pull-down convention where each node in the tree is located at the lowest possible generation, while all leaves are fixed at the zeroth generation. Formally:
\begin{align}
\mathrm{LCAG}_{ij}(\mathcal{G}) & = f\left ( \mathrm{LCA_{ij}\left ( \mathcal{G} \right ) }  \right ), \\
f\left ( u \right ) & = \begin{cases}0,& \text{if } u \text{ is a leaf} 
 \\\underset{v\in \mathcal{S}\left ( u \right ) }{\max}\left \{ f\left ( v \right ) \right \}+1, & \text{otherwise}
\end{cases}
\end{align}
where $\mathcal{S}\left ( u \right )$ is the set of children \sw{nodes} of \sw{the} node $u$.

\sw{The particle decay process and the LCAG matrix are illustrated in \Fref{task_study} (left) and \Fref{task_study} (right), respectively.}
% \Fref{task_study} shows an example of particle decay process (left), and the matrix represents its corresponding LCAG matrix (right). 
The LCAG matrix is an equivalent form of the adjacency matrix. \sw{Such a } form allows the same identifier to represent multiple ancestors and satisfies the requirements of permutation-aware and data representation size (only the number of leaf nodes is needed). This modification assumes that if there are structural rules that allow inferring the tree structure from only the leaf nodes, then these rules can also be used on the inferred structure to deduce the labels of unseen nodes, thus recovering the LCA and adjacency matrix. 

In the context of the particle decay process, if we know that some particles, for example, $a$ and $b$ come from the same parent node, we can add up \sw{the energies and momentum of }them to obtain the properties of the parent node. These properties can be used to reconstruct node labels in most cases. With the \sw{definition above}, we can convert LCAG from and to the adjacency matrix, so that we can obtain a rooted tree that is able to represent the entire physical process.

\subsection{Neural relational inference}\label{subsec:NRI}
Neural relational inference (NRI) was originally proposed by~\cite{NRI} as an unsupervised GNN with variational autoencoder structure. 
As a GNN model, NRI is capable of capturing inter-particle interactions in particle physics. In contrast to other GNNs, it provides more powerful relational modeling that improves the accuracy and efficiency of particle decay reconstruction. 

To obtain the initial representation of the edges, all nodes in the input graph passes through a node-to-edge layer, followed by a two-layer MLP. Then, to update the state embeddings between the edge-to-node and node-to-edge transformation layers, we employ a sequence of MLPs consisting of two linear layers with ELU activation and batch normalization. The NRI block contains an edge-to-node layer and a node-to-edge layer, and the number of MLPs within the NRI block and at the beginning and end of the model can be configured to improve its learning capability.
The state embedding of all connected edges in the graph is updated \sw{as follows} (we adopt the notation of~\cite{LCAG}):

\begin{align}
\mathrm{node-to-edge}:h_{(i,j)}^{l} & = f_{e}^{l}\left ( \left [ h_{i}^{l},h_{j}^{l} \right ]  \right ),   \\
\mathrm{edge-to-node}:h_{i}^{l+1} & = f_{v}^{l}\left ( \sum_{j}^{}h_{(i,j)}^{l}\right ),
\end{align}

\noindent where $h_{i}^{l}$ represents the hidden state of node $i$ at layer $l$, and $h_{(i,j)}^{l}$ represents the hidden state for the edge connecting nodes $i$ and $j$. The feedforward neural networks $f_e$ and $f_v$ are used to generate edge and node embeddings.
